# Supplementary material for: Enhanced Hallucination Detection in Neural Machine Translation through Simple Detector Aggregation
Source: arXiv:2402.13331 source file (2024-02-20)
Supplement: Supplementary file 1 [file appendix.tex]

\appendix

\section{Additional Results on Out-of-distribution Detection}
\label{sec:appendix}

\begin{table}[t]
\centering

\footnotesize
\begin{tabular}{>{\arraybackslash}m{2.45cm} r r}
\toprule
\textsc{Detector} & AUROC $\uparrow$ & FPR@90TPR $\uparrow$\\
\midrule \midrule
\multicolumn{3}{c}{{\textit{Individual Detectors}}} \\\midrule
\multicolumn{3}{l}{{\textit{External}}} \\
CometKiwi & 91.36 & 27.17 \\
LaBSE & 81.19 & 53.72 \\
\cdashlinelr{1-3}\noalign{\vskip 0.5ex}
\multicolumn{3}{l}{{\textit{Model-based}}} \\
Seq-Logprob & 68.26 & 74.65 \\
ALTI+ & 71.39 & 76.63 \\
Wass-Combo & 82.07 & 44.28 \\
\midrule\midrule
\multicolumn{3}{c}{{\textit{Aggregated Detectors}}} \\\midrule
\multicolumn{3}{l}{{\textit{External Only}}} \\
Isolation Forest & 85.58 & 45.07 \\
Max-Norm & 88.18 & 33.16 \\
Sum-Norm & 89.86 & 29.02 \\
\cdashlinelr{1-3}\noalign{\vskip 0.5ex}
\multicolumn{3}{l}{{\textit{Model-based Only}}} \\
Isolation Forest & 77.51 & 67.78 \\
Max-Norm & 70.46 & 75.51 \\
Sum-Norm & 78.71 & 55.84 \\
\cdashlinelr{1-3}\noalign{\vskip 0.5ex}
\multicolumn{3}{l}{{\textit{All}}} \\
Isolation Forest & 83.78 & 46.01 \\
Max-Norm & 87.16 & 31.87 \\
Sum-Norm & 88.02 & 26.81 \\
\bottomrule
\end{tabular}
\caption{is\_osc}
\label{tab:auroc_fpr_all}
\end{table}
\begin{table}[t]
\centering

\footnotesize
\begin{tabular}{>{\arraybackslash}m{2.45cm} r r}
\toprule
\textsc{Detector} & AUROC $\uparrow$ & FPR@90TPR $\uparrow$\\
\midrule \midrule
\multicolumn{3}{c}{{\textit{Individual Detectors}}} \\\midrule
\multicolumn{3}{l}{{\textit{External}}} \\
CometKiwi & 85.30 & 37.02 \\
LaBSE & 98.05 & 2.13 \\
\cdashlinelr{1-3}\noalign{\vskip 0.5ex}
\multicolumn{3}{l}{{\textit{Model-based}}} \\
Seq-Logprob & 94.22 & 6.84 \\
ALTI+ & 98.21 & 2.15 \\
Wass-Combo & 95.54 & 5.52 \\
\midrule\midrule
\multicolumn{3}{c}{{\textit{Aggregated Detectors}}} \\\midrule
\multicolumn{3}{l}{{\textit{External Only}}} \\
Isolation Forest & 97.96 & 3.11 \\
Max-Norm & 94.71 & 16.41 \\
Sum-Norm & 96.56 & 7.53 \\
\cdashlinelr{1-3}\noalign{\vskip 0.5ex}
\multicolumn{3}{l}{{\textit{Model-based Only}}} \\
Isolation Forest & 95.00 & 7.71 \\
Max-Norm & 97.09 & 1.70 \\
Sum-Norm & 98.23 & 1.97 \\
\cdashlinelr{1-3}\noalign{\vskip 0.5ex}
\multicolumn{3}{l}{{\textit{All}}} \\
Isolation Forest & 97.57 & 3.94 \\
Max-Norm & 95.11 & 14.53 \\
Sum-Norm & 98.34 & 2.21 \\
\bottomrule
\end{tabular}
\caption{is\_fd}
\label{tab:auroc_fpr_all}
\end{table}
\begin{table}[t]
\centering

\footnotesize
\begin{tabular}{>{\arraybackslash}m{2.45cm} r r}
\toprule
\textsc{Detector} & AUROC $\uparrow$ & FPR@90TPR $\uparrow$\\
\midrule \midrule
\multicolumn{3}{c}{{\textit{Individual Detectors}}} \\\midrule
\multicolumn{3}{l}{{\textit{External}}} \\
CometKiwi & 78.90 & 46.37 \\
LaBSE & 85.80 & 32.53 \\
\cdashlinelr{1-3}\noalign{\vskip 0.5ex}
\multicolumn{3}{l}{{\textit{Model-based}}} \\
Seq-Logprob & 77.85 & 66.95 \\
ALTI+ & 73.76 & 89.43 \\
Wass-Combo & 75.69 & 68.91 \\
\midrule\midrule
\multicolumn{3}{c}{{\textit{Aggregated Detectors}}} \\\midrule
\multicolumn{3}{l}{{\textit{External Only}}} \\
Isolation Forest & 85.10 & 38.27 \\
Max-Norm & 85.81 & 34.04 \\
Sum-Norm & 85.01 & 30.86 \\
\cdashlinelr{1-3}\noalign{\vskip 0.5ex}
\multicolumn{3}{l}{{\textit{Model-based Only}}} \\
Isolation Forest & 82.79 & 48.82 \\
Max-Norm & 74.45 & 83.14 \\
Sum-Norm & 80.70 & 69.87 \\
\cdashlinelr{1-3}\noalign{\vskip 0.5ex}
\multicolumn{3}{l}{{\textit{All}}} \\
Isolation Forest & 87.54 & 28.97 \\
Max-Norm & 84.06 & 43.87 \\
Sum-Norm & 86.65 & 35.04 \\
\bottomrule
\end{tabular}
\caption{is\_sd}
\label{tab:auroc_fpr_all}
\end{table}

\begin{table}[t]
\centering

\footnotesize
\begin{tabular}{>{\arraybackslash}m{2.45cm} r r}
\toprule
\textsc{Detector} & AUROC $\uparrow$ & FPR@90TPR $\uparrow$\\
\midrule \midrule
\multicolumn{3}{c}{{\textit{Individual Detectors}}} \\\midrule
\multicolumn{3}{l}{{\textit{External}}} \\
score\_comet\_qe & 82.71 & 46.13 \\
score\_labse & 88.96 & 34.92 \\
score\_laser & 81.12 & 46.81 \\
score\_xnli & 82.90 & 32.64 \\
\cdashlinelr{1-3}\noalign{\vskip 0.5ex}
\multicolumn{3}{l}{{\textit{Model-based}}} \\
score\_log\_loss & 86.58 & 28.37 \\
score\_alti\_mean & 82.18 & 58.76 \\
score\_attn\_ot & 64.95 & 84.66 \\
\midrule\midrule
\multicolumn{3}{c}{{\textit{Aggregated Detectors}}} \\\midrule
\multicolumn{3}{l}{{\textit{External Only}}} \\
Isolation Forest & 68.06 & 69.09 \\
Max-Norm & 89.25 & 32.10 \\
Sum-Norm & 89.89 & 32.58 \\
\cdashlinelr{1-3}\noalign{\vskip 0.5ex}
\multicolumn{3}{l}{{\textit{Model-based Only}}} \\
Isolation Forest & 72.18 & 76.33 \\
Max-Norm & 69.41 & 81.96 \\
Sum-Norm & 89.68 & 33.32 \\
\cdashlinelr{1-3}\noalign{\vskip 0.5ex}
\multicolumn{3}{l}{{\textit{All}}} \\
Isolation Forest & 74.72 & 64.27 \\
Max-Norm & 81.76 & 36.87 \\
Sum-Norm & 91.17 & 28.96 \\
\bottomrule
\end{tabular}
\caption{high Halomi is\_hall}
\label{tab:auroc_fpr_all}
\end{table}
\begin{table}[t]
\centering

\footnotesize
\begin{tabular}{>{\arraybackslash}m{2.45cm} r r}
\toprule
\textsc{Detector} & AUROC $\uparrow$ & FPR@90TPR $\uparrow$\\
\midrule \midrule
\multicolumn{3}{c}{{\textit{Individual Detectors}}} \\\midrule
\multicolumn{3}{l}{{\textit{External}}} \\
score\_comet\_qe & 73.35 & 65.81 \\
score\_labse & 84.67 & 38.75 \\
score\_laser & 75.51 & 52.70 \\
score\_xnli & 83.97 & 54.60 \\
\cdashlinelr{1-3}\noalign{\vskip 0.5ex}
\multicolumn{3}{l}{{\textit{Model-based}}} \\
score\_log\_loss & 78.31 & 54.55 \\
score\_alti\_mean & 68.51 & 79.30 \\
score\_attn\_ot & 66.65 & 84.17 \\
\midrule\midrule
\multicolumn{3}{c}{{\textit{Aggregated Detectors}}} \\\midrule
\multicolumn{3}{l}{{\textit{External Only}}} \\
Isolation Forest & 64.61 & 74.09 \\
Max-Norm & 85.71 & 37.90 \\
Sum-Norm & 85.99 & 38.43 \\
\cdashlinelr{1-3}\noalign{\vskip 0.5ex}
\multicolumn{3}{l}{{\textit{Model-based Only}}} \\
Isolation Forest & 61.09 & 88.40 \\
Max-Norm & 75.74 & 67.87 \\
Sum-Norm & 78.31 & 64.85 \\
\cdashlinelr{1-3}\noalign{\vskip 0.5ex}
\multicolumn{3}{l}{{\textit{All}}} \\
Isolation Forest & 67.02 & 74.66 \\
Max-Norm & 85.48 & 52.41 \\
Sum-Norm & 85.72 & 41.94 \\
\bottomrule
\end{tabular}
\caption{high Halomi is\_omit}
\label{tab:auroc_fpr_all}
\end{table}

\section{Additional Experimental Details}

\begin{table}[t]
\centering

\footnotesize
\begin{tabular}{>{\arraybackslash}m{2.45cm} r r}
\toprule
\textsc{Detector} & AUROC $\uparrow$ & FPR@90TPR $\uparrow$\\
\midrule \midrule
\multicolumn{3}{c}{{\textit{Individual Detectors}}} \\\midrule
\multicolumn{3}{l}{{\textit{External}}} \\
CometKiwi & 86.96 & 35.15 \\
LaBSE & 91.72 & 26.86 \\
\cdashlinelr{1-3}\noalign{\vskip 0.5ex}
\multicolumn{3}{l}{{\textit{Model-based}}} \\
Seq-Logprob & 83.40 & 58.99 \\
ALTI+ & 84.24 & 66.19 \\
Wass-Combo & 87.02 & 48.38 \\
\midrule\midrule
\multicolumn{3}{c}{{\textit{Aggregated Detectors}}} \\\midrule
\multicolumn{3}{l}{{\textit{External Only}}} \\
Isolation Forest & 93.06 & 16.40 \\
Max-Norm & 92.43 & 22.09 \\
Sum-Norm & 93.32 & 20.67 \\
\cdashlinelr{1-3}\noalign{\vskip 0.5ex}
\multicolumn{3}{l}{{\textit{Model-based Only}}} \\
Isolation Forest & 85.75 & 56.44 \\
Max-Norm & 83.81 & 62.94 \\
Sum-Norm & 89.07 & 42.50 \\
\cdashlinelr{1-3}\noalign{\vskip 0.5ex}
\multicolumn{3}{l}{{\textit{All}}} \\
Isolation Forest & \textbf{94.11} & \textbf{18.17} \\
Max-Norm & 91.60 & 26.38 \\
Sum-Norm & \textbf{94.12} & \textbf{17.06} \\
\bottomrule
\end{tabular}
\caption{is\_hall}
\label{tab:auroc_fpr_all}
\end{table}

\begin{table}[t]
\centering

\footnotesize
\begin{tabular}{>{\arraybackslash}m{2.45cm} r r}
\toprule
\textsc{Detector} & AUROC $\uparrow$ & FPR@90TPR $\uparrow$\\
\midrule \midrule
\multicolumn{3}{c}{{\textit{Individual Detectors}}} \\\midrule
\multicolumn{3}{l}{{\textit{External}}} \\
CometKiwi & \textbf{91.36} & \textbf{27.17} \\
LaBSE & 81.19 & 53.72 \\
\cdashlinelr{1-3}\noalign{\vskip 0.5ex}
\multicolumn{3}{l}{{\textit{Model-based}}} \\
Seq-Logprob & 68.26 & 74.65 \\
ALTI+ & 71.39 & 76.63 \\
Wass-Combo & 82.07 & 44.28 \\
\midrule\midrule
\multicolumn{3}{c}{{\textit{Aggregated Detectors}}} \\\midrule
\multicolumn{3}{l}{{\textit{External Only}}} \\
Isolation Forest & 88.78 & 36.53 \\
Max-Norm & 88.18 & 33.16 \\
Sum-Norm & \textbf{89.86} & 29.02 \\
\cdashlinelr{1-3}\noalign{\vskip 0.5ex}
\multicolumn{3}{l}{{\textit{Model-based Only}}} \\
Isolation Forest & 68.15 & 81.14 \\
Max-Norm & 70.46 & 75.51 \\
Sum-Norm & 78.71 & 55.84 \\
\cdashlinelr{1-3}\noalign{\vskip 0.5ex}
\multicolumn{3}{l}{{\textit{All}}} \\
Isolation Forest & 86.60 & 32.17 \\
Max-Norm & 87.16 & 31.87 \\
Sum-Norm & 88.02 & \textbf{26.81} \\
\bottomrule
\end{tabular}
\caption{is\_osc}
\label{tab:auroc_fpr_all}
\end{table}

\begin{table}[t]
\centering

\footnotesize
\begin{tabular}{>{\arraybackslash}m{2.45cm} r r}
\toprule
\textsc{Detector} & AUROC $\uparrow$ & FPR@90TPR $\uparrow$\\
\midrule \midrule
\multicolumn{3}{c}{{\textit{Individual Detectors}}} \\\midrule
\multicolumn{3}{l}{{\textit{External}}} \\
CometKiwi & 85.30 & 37.02 \\
LaBSE & 98.05 & 2.13 \\
\cdashlinelr{1-3}\noalign{\vskip 0.5ex}
\multicolumn{3}{l}{{\textit{Model-based}}} \\
Seq-Logprob & 94.22 & 6.84 \\
ALTI+ & 98.21 & 2.15 \\
Wass-Combo & 95.54 & 5.52 \\
\midrule\midrule
\multicolumn{3}{c}{{\textit{Aggregated Detectors}}} \\\midrule
\multicolumn{3}{l}{{\textit{External Only}}} \\
Isolation Forest & 94.48 & 13.83 \\
Max-Norm & 94.71 & 16.41 \\
Sum-Norm & 96.56 & 7.53 \\
\cdashlinelr{1-3}\noalign{\vskip 0.5ex}
\multicolumn{3}{l}{{\textit{Model-based Only}}} \\
Isolation Forest & 97.49 & 2.14 \\
Max-Norm & 97.09 & 1.70 \\
Sum-Norm & 98.23 & 1.97 \\
\cdashlinelr{1-3}\noalign{\vskip 0.5ex}
\multicolumn{3}{l}{{\textit{All}}} \\
Isolation Forest & 97.63 & 4.99 \\
Max-Norm & 95.11 & 14.53 \\
Sum-Norm & \textbf{98.34} & 2.21 \\
\bottomrule
\end{tabular}
\caption{is\_fd}
\label{tab:auroc_fpr_all}
\end{table}

\begin{table}[t]
\centering

\footnotesize
\begin{tabular}{>{\arraybackslash}m{2.45cm} r r}
\toprule
\textsc{Detector} & AUROC $\uparrow$ & FPR@90TPR $\uparrow$\\
\midrule \midrule
\multicolumn{3}{c}{{\textit{Individual Detectors}}} \\\midrule
\multicolumn{3}{l}{{\textit{External}}} \\
CometKiwi & 78.90 & 46.37 \\
LaBSE & 85.80 & 32.53 \\
\cdashlinelr{1-3}\noalign{\vskip 0.5ex}
\multicolumn{3}{l}{{\textit{Model-based}}} \\
Seq-Logprob & 77.85 & 66.95 \\
ALTI+ & 73.76 & 89.43 \\
Wass-Combo & 75.69 & 68.91 \\
\midrule\midrule
\multicolumn{3}{c}{{\textit{Aggregated Detectors}}} \\\midrule
\multicolumn{3}{l}{{\textit{External Only}}} \\
Isolation Forest & 86.82 & 30.41 \\
Max-Norm & 85.81 & 34.04 \\
Sum-Norm & 85.01 & 30.86 \\
\cdashlinelr{1-3}\noalign{\vskip 0.5ex}
\multicolumn{3}{l}{{\textit{Model-based Only}}} \\
Isolation Forest & 79.96 & 60.54 \\
Max-Norm & 74.45 & 83.14 \\
Sum-Norm & 80.70 & 69.87 \\
\cdashlinelr{1-3}\noalign{\vskip 0.5ex}
\multicolumn{3}{l}{{\textit{All}}} \\
Isolation Forest & \textbf{88.05} & \textbf{29.71} \\
Max-Norm & 84.06 & 43.87 \\
Sum-Norm & 86.65 & 35.04 \\
\bottomrule
\end{tabular}
\caption{is\_sd}
\label{tab:auroc_fpr_all}
\end{table}

\begin{table}[t]
\centering

\footnotesize
\begin{tabular}{>{\arraybackslash}m{2.45cm} r r}
\toprule
\textsc{Detector} & AUROC $\uparrow$ & FPR@90TPR $\downarrow$\\
\midrule \midrule
\multicolumn{3}{c}{{\textit{Individual Detectors}}} \\\midrule
\multicolumn{3}{l}{{\textit{External}}} \\
COMET-QE & 73.41 & 50.40 \\
LaBSE & \textbf{85.91} & \textbf{40.33} \\
LASER & 76.22 & 57.17 \\
XNLI & 75.33 & 45.47 \\
\cdashlinelr{1-3}\noalign{\vskip 0.5ex}
\multicolumn{3}{l}{{\textit{Model-based}}} \\
Seq-Logprob & 80.64 & 49.37 \\
ALTI & 77.45 & 60.82 \\
Attn-OT & 63.93 & 84.80 \\
\midrule\midrule
\multicolumn{3}{c}{{\textit{Aggregated Detectors}}} \\\midrule
\multicolumn{3}{l}{{\textit{External Only}}} \\
Isolation Forest & \dab{40.94} 44.97 & \daglb{55.99} 96.32 \\
Sum-Norm & \dab{0.5} 85.41 & \daglb{0.5} 40.83 \\
\cdashlinelr{1-3}\noalign{\vskip 0.5ex}
\multicolumn{3}{l}{{\textit{Model-based Only}}} \\
Isolation Forest & \dab{20.05} 65.86 & \daglb{40.65} 80.98 \\
Sum-Norm & \dab{2.01} 83.90 & \daglb{6.04} 46.37 \\
\cdashlinelr{1-3}\noalign{\vskip 0.5ex}
\multicolumn{3}{l}{{\textit{All}}} \\
Isolation Forest & \dab{32.75} 53.16 & \daglb{52.62} 92.92 \\
Sum-Norm & \uag{1.15} \textbf{87.06} & \uaglb{2.00} \textbf{38.33} \\
\bottomrule
\end{tabular}
\caption{Performance of all hallucination detectors on the HalOmi Dataset}
\label{tab:auroc_fpr_all}
\end{table}
% note : the IF fails because the proportions of hallucinations in the HalOmi dataset is 34% which is a lot

\begin{figure}[h!]
    \centering
        \includegraphics[width=0.4\textwidth]{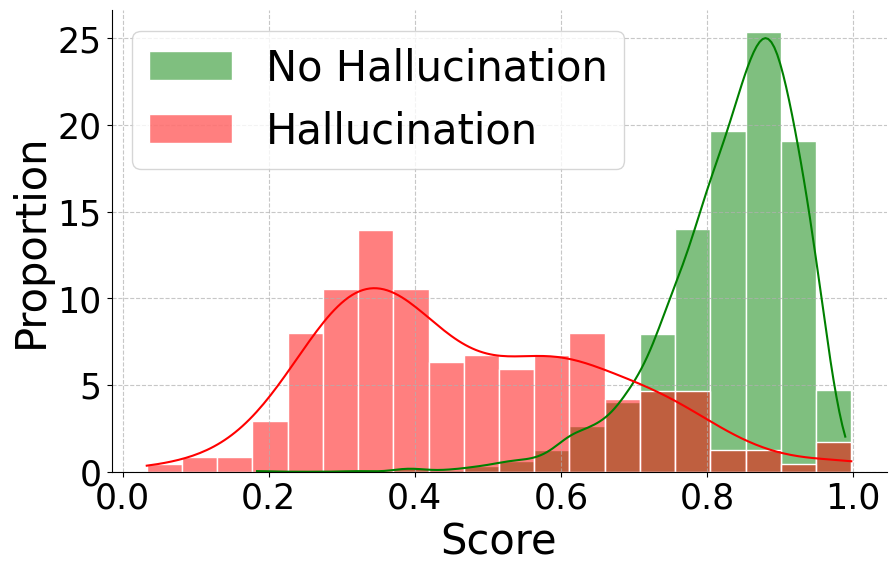}
        \includegraphics[width=0.4\textwidth]{images/labse_pred2.png}
        \caption{LaBSE}
        \label{fig:subfig1}
    \end{figure}
